# Supplementary material for: Nonlinear spontaneous flow instability in active nematics
Source: arXiv:2403.16841 source file (2024-03-25)
Supplement: Supplementary file 1 [file SM.pdf]

# Supplemental Material for Nonlinear spontaneous flow instability in active nematics

Ido Lavi,<sup>1,2</sup> Ricard Alert,<sup>3,4,5</sup> Jean-François Joanny,<sup>6,7</sup> and Jaume Casademunt<sup>1</sup>

<sup>1</sup>*Departament de Física de la Matèria Condensada,  
Universitat de Barcelona, Martí i Franquès 1, 08028 Barcelona, Spain,  
and UBICS (University of Barcelona Institute of Complex Systems)*

<sup>2</sup>*Center for Computational Biology, Flatiron Institute, 162 5th Ave, New York, NY 10010, USA*

<sup>3</sup>*Max Planck Institute for the Physics of Complex Systems, Nöthnitzerst. 38, 01187 Dresden, Germany*

<sup>4</sup>*Center for Systems Biology Dresden, Pfotenhauerst. 108, 01307 Dresden, Germany*

<sup>5</sup>*Cluster of Excellence Physics of Life, TU Dresden, 01062 Dresden, Germany*

<sup>6</sup>*Collège de France, Paris, France*

<sup>7</sup>*Laboratoire PhysicoChimie Curie, Institut Curie,  
Université Paris Sciences & Lettres (PSL), Sorbonne Universités, Paris, France*

## S.1. REDUCED EQUATIONS

Here we provide a brief derivation of the reduced  $\theta$  and  $\psi$  equations, including adimensionalized forms. With the Frank energy  $F_n$  as defined in Eq. (1), one has

$$h_\alpha = -\frac{\delta F_n}{\delta n_\alpha} = K \nabla^2 n_\alpha + h_\parallel^0 n_\alpha. \quad (\text{S.1})$$

Substituting  $\mathbf{n} = (\cos \theta, \sin \theta)$ ,

$$h_\parallel = \mathbf{n} \cdot \mathbf{h} = -K(\partial_x \theta)^2 - K(\partial_y \theta)^2 + h_\parallel^0, \quad h_\perp = \mathbf{n}_\perp \cdot \mathbf{h} = K \nabla^2 \theta. \quad (\text{S.2})$$

where  $\mathbf{n}_\perp = (-\sin \theta, \cos \theta)$ . The nematic torque  $h_\perp$  is fully defined by Eq. (S.2), but the Lagrange multiplier  $h_\parallel^0$  is yet to be determined.

We now substitute  $\mathbf{n} = (\cos \theta, \sin \theta)$  in Eq. (2) and separate the parallel and perpendicular components:

$$0 = \frac{h_\parallel}{\gamma} - \nu(\partial_\alpha v_\beta) q_{\alpha\beta}, \quad (\text{S.3})$$

$$\partial_t \theta + v_\alpha \partial_\alpha \theta - \frac{1}{2} \omega = \frac{h_\perp}{\gamma} - \nu(\partial_\alpha v_\beta) \bar{q}_{\alpha\beta}. \quad (\text{S.4})$$

where  $\omega = \partial_x v_y - \partial_y v_x$  and  $\bar{q}_{\alpha\beta} = -\varepsilon_{\alpha\gamma} q_{\gamma\beta}$ , with  $\varepsilon$  the Levi-Civita tensor. In terms of  $\psi$  and  $\theta$ ,

$$v_\alpha = \varepsilon_{\alpha\beta} \partial_\beta \psi, \quad \partial_\alpha v_\beta = \varepsilon_{\beta\gamma} \partial_\alpha \partial_\gamma \psi, \quad \omega = -\nabla^2 \psi, \quad q = \frac{1}{2} \begin{pmatrix} \cos 2\theta & \sin 2\theta \\ \sin 2\theta & -\cos 2\theta \end{pmatrix}, \quad \bar{q} = \frac{1}{2} \begin{pmatrix} -\sin 2\theta & \cos 2\theta \\ \cos 2\theta & \sin 2\theta \end{pmatrix}.$$

Equation (S.3) directly defines  $h_\parallel$  (and  $h_\parallel^0$  by extension) while Eq. (S.4) prescribes the evolution of  $\theta$ .

As for the momentum balance, we take the curl of Eq. (3) to obtain a scalar equation for  $\psi$ :

$$0 = -\eta \nabla^4 \psi - \varepsilon_{\alpha\beta} (\partial_\alpha h_\perp) \partial_\beta \theta - \frac{1}{2} \nabla^2 h_\perp - \nu \partial_\alpha \partial_\beta (\bar{q}_{\alpha\beta} h_\parallel - q_{\alpha\beta} h_\perp) + \zeta \partial_\alpha \partial_\beta \bar{q}_{\alpha\beta}. \quad (\text{S.5})$$

Recall here that  $h_\parallel$  is also function of  $\psi$  (see Eq. (S.3)). This property of the model makes the finite  $\nu$  scenario considerably more intricate compared to the special  $\nu = 0$  case [1].

The adimensionalized equations in terms of  $S = \zeta/|\zeta|$ ,  $R = \eta/\gamma$ ,  $\nu$ , and  $A = R|\zeta|L^2/K$  reduce to

$$\partial_t \theta + \varepsilon_{\alpha\beta} (\partial_\beta \psi) \partial_\alpha \theta + \frac{1}{2} \nabla^2 \psi = \frac{1}{A} \nabla^2 \theta + \nu (\partial_\alpha \partial_\beta \psi) q_{\alpha\beta}, \quad (\text{S.6})$$

$$\nabla^4 \psi + \frac{R}{A} \varepsilon_{\alpha\beta} (\partial_\alpha \nabla^2 \theta) \partial_\beta \theta + \frac{R}{2A} \nabla^4 \theta + R \nu \partial_\alpha \partial_\beta \left( \nu \bar{q}_{\alpha\beta} (\partial_i \partial_j \psi) \bar{q}_{ij} - q_{\alpha\beta} \frac{1}{A} \nabla^2 \theta \right) = S \partial_\alpha \partial_\beta \bar{q}_{\alpha\beta}. \quad (\text{S.7})$$

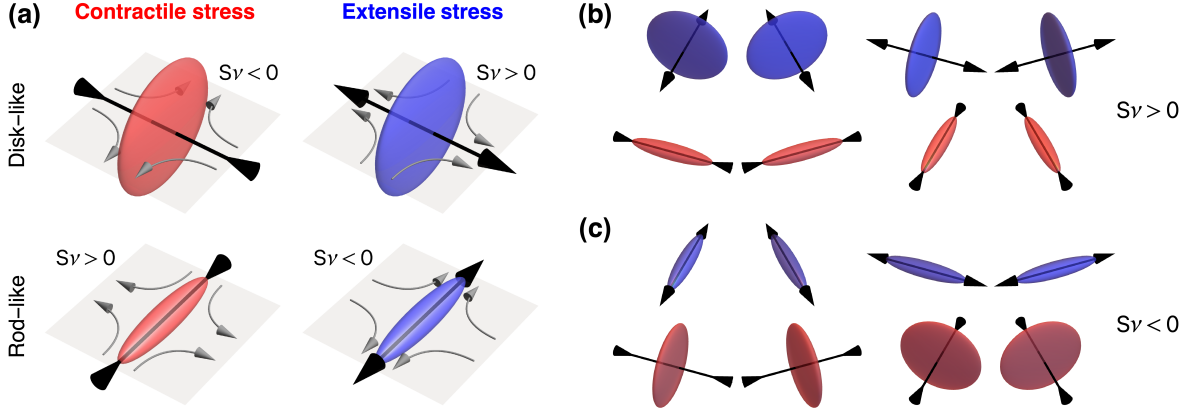

FIG. S.1. **Illustration of the activity-alignment symmetry.** (a) Gray streams illustrate the two-dimensional flow induced by a contractile ( $S = -1$ , red) or extensile ( $S = +1$ , blue) particle with respect to its nematic orientation ( $\pm \mathbf{n}$ , black). Rod-like alignment ( $\nu < 0$ ) means that the long axis of particles is aligned with  $\mathbf{n}$ , whereas disk-like alignment ( $\nu > 0$ ) implies that the long axis is perpendicular to  $\mathbf{n}$ . What matters physically is how the active stress is oriented with respect to the long axis. (b) Extensile disk-like and contractile rod-like systems ( $S\nu > 0$ ) are equivalent in 2D, upon a  $90^\circ$  rotation of the director. In the one-constant approximation, splaying the director in one case is equivalent to bending the director in the other. (c) The same equivalence holds between extensile rod-like and contractile disk-like systems ( $S\nu < 0$ ).

## S.2. ACTIVITY-ALIGNMENT SYMMETRY

Here we elaborate on the invariance of our equations of motion under the activity-alignment transformation  $(S, A, R, \nu, \theta) \rightarrow (-S, A, R, -\nu, \theta + \pi/2)$ . This symmetry has been noted in the past [2, 3] and is reflected in Figs. 1–3. Following the rotation  $\theta \rightarrow \theta + \pi/2$ , one has:

$$\partial_t \theta \rightarrow \partial_t \theta, \partial_\alpha \theta \rightarrow \partial_\alpha \theta, q \rightarrow -q, \bar{q} \rightarrow -\bar{q}.$$

With this transformation, it is easy to see how Eqs. (S.6),(S.7) remain unchanged if  $\nu \rightarrow -\nu$  and  $S \rightarrow -S$ .

In Fig. S.1, we demonstrate the underlying reason for this symmetry. For a 2D system (gray surfaces in Fig. S.1(a)), disk-like flow alignment ( $\nu > 0$ ) implies that the long axis of particles is perpendicular to  $\mathbf{n}$ , unlike with rods where it is parallel to  $\mathbf{n}$  ( $\nu < 0$ ). Thus, the passive interaction between particles and the fluid remains the same after reversing the sign of  $\nu$  and rotating all particles by  $90^\circ$ . Likewise, contractile and extensile stresses become equivalent under the same rotation. Consequently, splaying (bending) of extensile disk-like particles is equivalent to bending (splaying) of contractile rods (Fig. S.1(b)). Similarly, splaying (bending) of extensile rod-like particles corresponds to bending (splaying) of contractile disks (Fig. S.1(c)).

### S.3. WEAKLY NONLINEAR ANALYSIS

Here we analyze the weakly nonlinear response to orientational perturbations about the uniform quiescent state. Aside from deriving the linear growth rate, we aim to characterize the critical nature of the bifurcation. Starting from the base state,  $\theta(\mathbf{r}) = 0$ , we consider the perturbation  $\delta\theta = \epsilon \cos(\mathbf{k} \cdot \mathbf{r})$ , with  $\mathbf{k} = k(\cos \phi, \sin \phi)$ .

Utilizing Mathematica (TM), we find the solution to Eq. (S.7) up to  $\epsilon^3$ :

$$\psi = a_1 \epsilon \cos(\mathbf{k} \cdot \mathbf{r}) + b_2 \epsilon^2 \cos(2\mathbf{k} \cdot \mathbf{r}) + c_1 \epsilon^3 \cos(\mathbf{k} \cdot \mathbf{r}) + c_3 \epsilon^3 \cos(3\mathbf{k} \cdot \mathbf{r}) + \mathcal{O}(\epsilon^4), \quad (\text{S.8})$$

where

$$\begin{aligned} a_1 &= \frac{2(2AS \cos 2\phi + k^2 R(\nu \cos 2\phi - 1))}{Ak^2(4 + R\nu^2 \sin^2 2\phi)}, \\ b_2 &= -\frac{(AS(8 + R\nu^2(5 + 3 \cos 4\phi)) + k^2 R\nu(8 - 4R\nu \cos 2\phi + R\nu^2(3 + \cos 4\phi))) \sin 2\phi}{4Ak^2(4 + R\nu^2 \sin^2 2\phi)^2}, \\ c_1 &= \frac{-1}{16Ak^2(4 + R\nu^2 \sin^2 2\phi)^3} \left( 4AS \cos 2\phi (128 + 192R\nu^2 \cos 4\phi + R^2\nu^4(-23 + 28 \cos 4\phi - 5 \cos 8\phi)) \right. \\ &\quad + k^2 R\nu \left( 768 \cos 2\phi - 384R\nu \cos 4\phi + R\nu^2(224 \cos 2\phi + 160 \cos 6\phi) + R^2\nu^3(40 - 48 \cos 4\phi + 8 \cos 8\phi) \right. \\ &\quad \left. \left. + R^2\nu^4(-18 \cos 2\phi + 23 \cos 6\phi - 5 \cos 10\phi) \right) \right), \\ c_3 &= \frac{-1}{432Ak^2(4 + R\nu^2 \sin^2 2\phi)^3} \left( 4AS \cos 2\phi (128 + R\nu^2(-64 + 256 \cos 4\phi) + R^2\nu^4(-51 + 44 \cos 4\phi + 7 \cos 8\phi)) \right. \\ &\quad + 3k^2 R\nu \left( 256 \cos 2\phi - 128R\nu \cos 4\phi + R\nu^2(32 \cos 2\phi + 96 \cos 6\phi) + R^2\nu^3(24 - 16 \cos 4\phi - 8 \cos 8\phi) \right. \\ &\quad \left. \left. + R^2\nu^4(-22 \cos 2\phi + 21 \cos 6\phi + \cos 10\phi) \right) \right). \end{aligned}$$

Specifically, for bend ( $\phi = 0$ ):

$$a_1 = \frac{S}{k^2} + \frac{R(\nu - 1)}{2A}, \quad b_2 = 0, \quad c_1 = -\frac{S(2 + 3R\nu^2)}{4k^2} - \frac{3R\nu(2 + R\nu(\nu - 1))}{8A}, \quad c_3 = \frac{1}{27}c_1,$$

and for splay ( $\phi = \pi/2$ ):

$$a_1 = -\frac{S}{k^2} - \frac{R(\nu + 1)}{2A}, \quad b_2 = 0, \quad c_1 = \frac{S(2 + 3R\nu^2)}{8k^2} + \frac{3R\nu(2 + R\nu(\nu + 1))}{8A}, \quad c_3 = \frac{1}{27}c_1.$$

Substituting  $\delta\theta$  and  $\psi$ , Eq. (S.8), back in Eq. (S.6) gives:

$$\partial_t \theta = \Omega_{2,0} \epsilon^2 + (\Omega_{1,1} \epsilon + \Omega_{3,1} \epsilon^3) \cos(\mathbf{k} \cdot \mathbf{r}) + \Omega_{2,2} \epsilon^2 \cos(2\mathbf{k} \cdot \mathbf{r}) + \Omega_{3,3} \epsilon^3 \cos(3\mathbf{k} \cdot \mathbf{r}) + \mathcal{O}(\epsilon^4), \quad (\text{S.9})$$

such that the lower first and second indices of the  $\Omega$  coefficients denote the power of  $\epsilon$  and the order of the harmonic, respectively. We obtain these analytically for all parameters and any  $k, \phi$ :

$$\begin{aligned}
\Omega_{2,0} &= -\frac{AS\nu \sin 4\phi + k^2 R\nu(-1 + \nu \cos 2\phi) \sin 2\phi}{A(4 + R\nu^2 \sin^2 2\phi)}, \\
\Omega_{1,1} &= \frac{2AS \cos 2\phi(1 - \nu \cos 2\phi) - k^2(4 + R + R\nu^2 - 2R\nu \cos 2\phi)}{A(4 + \nu^2 R \sin^2 2\phi)}, \\
\Omega_{3,1} &= \frac{1}{16A(4 + R\nu^2 \sin^2 2\phi)^3} \left( 2AS \left( -128 \cos 2\phi + 64\nu(3 + 5 \cos 4\phi) + 96R\nu^2(\cos 2\phi + \cos 6\phi) \right. \right. \\
&\quad \left. \left. - 32R\nu^3(1 + 4 \cos 4\phi + \cos 8\phi) + 2R^2\nu^4 \sin^2 2\phi(13 \cos 2\phi - 5 \cos 6\phi) - R^2\nu^5 \sin^2 2\phi(17 + 4 \cos 4\phi - 5 \cos 8\phi) \right) \right. \\
&\quad \left. - k^2 R\nu \left( 768 \cos 2\phi - \nu(256 + (512 + 192R) \cos 4\phi) + R\nu^2(224 \cos 2\phi + 160 \cos 6\phi) \right. \right. \\
&\quad \left. \left. + R\nu^3(-16 + 20R - (160 + 24R) \cos 4\phi + 4(-4 + R) \cos 8\phi) + R^2\nu^4(-18 \cos 2\phi + 23 \cos 6\phi - 5 \cos 10\phi) \right. \right. \\
&\quad \left. \left. + R^2\nu^5(10 - 9 \cos 4\phi - 2 \cos 8\phi + \cos 12\phi) \right) \right), \\
\Omega_{2,2} &= \frac{-1}{8A(4 + \nu^2 R \sin^2 2\phi)^2} \left( AS(-32 \sin 2\phi + 48\nu \sin 4\phi - R\nu^2(14 \sin 2\phi + 6 \sin 6\phi) + R\nu^3(14 \sin 4\phi + \sin 8\phi)) \right. \\
&\quad \left. - 16k^2 R\nu(1 - \nu \cos 2\phi)(4 + R\nu(\nu - \cos 2\phi)) \sin 2\phi \right), \\
\Omega_{3,3} &= \frac{1}{48A(4 + R\nu^2 \sin^2 2\phi)^3} \left( 2AS \left( -128 \cos 2\phi + 64\nu(1 + 7 \cos 4\phi) - 64R\nu^2(\cos 2\phi + 2 \cos 6\phi) \right. \right. \\
&\quad \left. \left. + 64R\nu^3(-1 + 3 \cos 4\phi + \cos 8\phi) + 2R^2\nu^4 \sin^2 \phi(65 \cos 2\phi + 7 \cos 6\phi) - R^2\nu^5 \sin^2 2\phi(83 + 60 \cos 4\phi + \cos 8\phi) \right) \right. \\
&\quad \left. - 3k^2 R\nu \left( 256 \cos 2\phi - 64\nu(4 + R) \cos 4\phi + 32R\nu^2(\cos 2\phi + 3 \cos 6\phi) + 4R\nu^3(3(4 + R) - 2(12 + R) \cos 4\phi \right. \right. \\
&\quad \left. \left. - (4 + R) \cos 8\phi) + R^2\nu^4(-22 \cos 2\phi + 21 \cos 6\phi + \cos 10\phi) + 4R^2\nu^5(3 - 2 \cos 4\phi - \cos 8\phi) \right) \right).
\end{aligned}$$

Here,  $\Omega_{1,1}$  corresponds to the linear growth rate, Eq. (4). Specifically, for bend ( $\phi = 0$ ):

$$\begin{aligned}
\Omega_{1,1} &= -\frac{k^2}{4A}(4 + R + R\nu^2 - 2R\nu) + \frac{1}{2}S(1 - \nu), \quad \Omega_{2,0} = 0, \quad \Omega_{2,2} = 0, \\
\Omega_{3,1} &= -\frac{3k^2}{16A}R\nu(1 - \nu)(4 - R\nu(1 - \nu)) - \frac{S}{8}(2 - 8\nu + 3R\nu^2(1 - \nu)), \quad \Omega_{3,3} = \frac{1}{3}\Omega_{3,1},
\end{aligned}$$

and for splay ( $\phi = \pi/2$ ):

$$\begin{aligned}
\Omega_{1,1} &= -\frac{k^2}{4A}(4 + R + R\nu^2 + 2R\nu) - \frac{1}{2}S(1 + \nu), \quad \Omega_{2,0} = 0, \quad \Omega_{2,2} = 0, \\
\Omega_{3,1} &= \frac{3k^2}{16A}R\nu(1 + \nu)(4 + R\nu(1 + \nu)) + \frac{S}{8}(2 + 8\nu + 3R\nu^2(1 + \nu)), \quad \Omega_{3,3} = \frac{1}{3}\Omega_{3,1}.
\end{aligned}$$

### A. Onset of the nonlinear instability

It follows from Eq. (S.9) and symmetry that  $\partial_t \epsilon = \Omega_{1,1}\epsilon + \Omega_{3,1}\epsilon^3 + \mathcal{O}(\epsilon^5)$ , as noted in the main text (Eq. (5)). Hence, the bifurcation occurring at  $\Omega_{1,1} = 0$  is supercritical if  $\Omega_{3,1} < 0$  and subcritical if  $\Omega_{3,1} > 0$ . For given  $S$  and  $R$ , the system of equations  $\Omega_{1,1} = 0$  &  $\Omega_{3,1} = 0$  define the tricritical point  $(\nu_\phi^*, A_\phi^*)$  at which the qualitative transition occurs. For arbitrary  $\phi$ , this boils down to

$$A_\phi^* = \frac{Sk^2(4 + R + R\nu_\phi^{*2} - 2R\nu_\phi^* \cos 2\phi)}{2 \cos 2\phi(1 - \nu_\phi^* \cos 2\phi)}, \quad (\text{S.10})$$

with  $\nu_\phi^*$  defined implicitly:

$$\begin{aligned}
0 = & -32(4 + R) \cos 2\phi + \nu_\phi^* (192 - 16R + 16(20 + R) \cos 4\phi) - R\nu_\phi^{*2} (2(12 - R)r \cos 2\phi + 2R(R + 36) \cos 6\phi) \\
& + R\nu_\phi^{*3} ((12 - 5R) + 4(24 + R) \cos 4\phi + (20 + R) \cos 8\phi) + 2R^2\nu_\phi^{*4} (5 \cos 2\phi - 6 \cos 6\phi + \cos 10\phi) \\
& + R^2\nu_\phi^{*5} (-7 + 5 \cos 4\phi + 3 \cos 8\phi - \cos 12\phi).
\end{aligned} \tag{S.11}$$

For bend ( $\phi = 0$ ) and for splay ( $\phi = \pi/2$ ), we find explicitly one real-valued root of Eq. (S.11):

$$\nu_0^* = \frac{1}{12} \left( 3 + \frac{3^{2/3}(-64 + 3R)}{\left( 81R^3 + 4\sqrt{3R^3(16384 + 9R(-256 + 3R(4 + 5R)))} \right)^{1/3}} \right) \tag{S.12}$$

$$\begin{aligned}
& + \frac{3^{1/3}}{R} \left( 81R^3 + 4\sqrt{3R^3(16384 + 9R(-256 + 3R(4 + 5R)))} \right)^{1/3} \Big), \\
\nu_{\pi/2}^* & = -\nu_0^*.
\end{aligned} \tag{S.13}$$

Due to the special symmetry in our problem,  $A^*$  is the same for the contractile splay mode ( $S = -1$ ,  $\phi = \pi/2$ ) and the extensile bend mode ( $S = +1$ ,  $\phi = 0$ ). For  $\nu/\nu^* > 1$  and  $A > A^*$ , the respective pitchfork bifurcation is subcritical. Specifically, for  $R = 1$  and  $S = -1$  we obtain  $(\nu_{\pi/2}^*, A_{\pi/2}^*) \simeq (-0.3267, 130.09)$ , marked by the filled magenta circle in Fig. 1(a) and Fig. 2(c). The analogous point for a bend perturbation in the extensile case ( $\nu_0^*, A_0^*$ ) is marked by the filled cyan circle in Fig. 1(b) and Fig. 2(d).

## B. Mean rotation

The rate  $\Omega_{2,0}$  defines how a sinusoidal perturbation engenders a second-order change in the mean orientation. This rotation arises in response to a flow-alignment torque associated with oblique perturbation modes:  $\phi \neq 0, \pi/2$ .

## C. Higher harmonic generation

The rates  $\Omega_{2,2}$  and  $\Omega_{3,3}$  define how a sinusoidal perturbation of the quiescent base state engenders its second and third  $\mathbf{k}$ -harmonics (at second-order and third-order in  $\epsilon$ , respectively). Note that  $\Omega_{2,2}$  is only at play for oblique angles, similar to  $\Omega_{2,0}$ . In principal, couplings to higher harmonics can be obtained by further expansion of  $\partial_t \theta$  in terms of  $\epsilon$ .

#### S.4. STRIPED SOLUTIONS (SHOOTING METHOD)

Here we outline our method for computing the quasi-1D steady states presented in Fig. 2. The steady,  $x$ -independent forms of Eqs. (S.6)–(S.7) are given by:

$$\frac{1}{2}\partial_y^2\psi = \frac{1}{A}\partial_y^2\theta - \frac{\nu}{2}\cos 2\theta \partial_y^2\psi, \quad (\text{S.14})$$

$$\partial_y^4\psi + \frac{R}{2A}\partial_y^4\theta + \frac{R\nu}{2}\partial_y^2\left(\frac{\nu}{2}\sin^2 2\theta \partial_y^2\psi + \frac{1}{A}\cos 2\theta \partial_y^2\theta\right) = \frac{S}{2}\partial_y^2\sin 2\theta. \quad (\text{S.15})$$

After integrating Eq. (S.15) twice and imposing periodic BCs, one has

$$\partial_y^2\psi + \frac{R}{2A}\partial_y^2\theta + \frac{R\nu}{2}\left(\frac{\nu}{2}\sin^2 2\theta \partial_y^2\psi + \frac{1}{A}\cos 2\theta \partial_y^2\theta\right) = \frac{S}{2}\sin 2\theta - \frac{S}{2}\sin 2\theta_0, \quad (\text{S.16})$$

where the last term on the RHS is an integration constant, chosen such that the uniform state  $\theta = \theta_0$  remains a quiescent solution.

It follows from Eq. (S.14) that

$$\partial_y^2\psi = \frac{2\partial_y^2\theta}{A(1 + \nu\cos 2\theta)}. \quad (\text{S.17})$$

Substituting Eq. (S.17) in Eq. (S.16) gives a closed ODE for  $\theta$ :

$$(4 + R + R\nu^2 + 2R\nu\cos 2\theta) \partial_y^2\theta = AS(1 + \nu\cos 2\theta)(\sin 2\theta - \sin 2\theta_0), \quad (\text{S.18})$$

equivalent to Eq. (6) in the main text.

We implemented the following algorithm for finding the solutions of interest to Eq. (S.18):

- To obtain a pattern of wavelength  $\lambda = 1$ , we begin by estimating a guess for the saturation angle  $\theta_{\text{sat}}$ . To this end, we employ a parametric continuation scheme: for a new iteration of the varied parameter (in our case  $\nu$ ), an estimate of  $\theta_{\text{sat}}$  is extrapolated from the previously registered results.
- Generate a list of angles  $\{\theta^i\}$  that span a narrow range about the initial guess.
- For all entries in  $\{\theta^i\}$ , we use the ODE solver in Mathematica (**NDSolve** with default settings) to compute solutions of Eq. (S.18) with the following BCs:

$$\theta(0) = \theta^i, \quad \theta'(0) = 0.$$

- For each numerical solution, verify that  $k = 2\pi$  is the dominant mode:  $\theta(y)$  should have one minima about  $y = 0.5$ . Then register the resulting value for  $\Delta\theta^i := \theta^i - \theta(1)$ . For a proper estimation range, and granted that a solution exists, this series crosses zero once, and perhaps twice (in the vicinity of a saddle-node). If this series is both nonmonotonic and does not cross zero, we infer the absence of a solution for the given parameters.
- Define a first-order polynomial interpolation of the list  $\{\theta^i, \Delta\theta^i\}$  and find its root  $\theta^*$ .
- Compute the solution to Eq. (S.18) with the following BCs:

$$\theta(0) = \theta^*, \quad \theta'(0) = 0.$$

If  $|\Delta\theta^*| = |\theta^* - \theta(1)| < \varepsilon$  (with  $\varepsilon$  a small computational tolerance, typically  $10^{-7}$ ), register  $\theta^*$  as the amplitude of the solution. Otherwise, repeat these steps with a refined guessing range about  $\theta^*$ .

- Based on all registered results, update the interpolation of  $\theta^*(\nu)$ . Lastly, iterate  $\nu$  with the other parameters fixed.

This procedure may be tricky and sensitive in some limits, e.g. next to bifurcations. Notwithstanding, it is a highly effective tool with which we were able to trace out the stable and unstable solution branches.

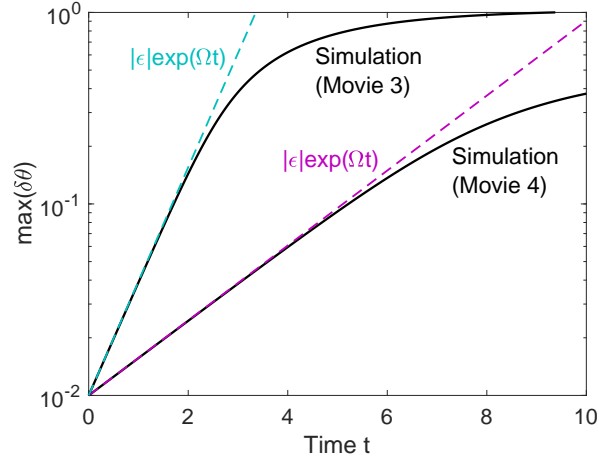

FIG. S.2. **Simulations vs linear stability analysis.** Black lines correspond to the max deviation from the quiescent state,  $\delta\theta$ , as a function of time in our numerical simulations (see Movies 3–4 with corresponding captions). Dashed cyan (magenta) line depicts the exponential growth of a bend (splay) modulation as determined by the linear growth rate  $\Omega$ , Eq. (4). Parameters were fixed as in Fig. 2(b).

### S.5. DYNAMIC SIMULATIONS (PSEUDOSPECTRAL SCHEME)

Here we outline our numerical integration method for demonstrating the stability/instability of our nonlinear steady states. Solutions obtained through this method are depicted in Movies 1–4.

The time-dependent,  $x$ -independent form of Eq. (S.6) reads:

$$\partial_t \theta = \frac{1}{A} \partial_y^2 \theta - \frac{1}{2} (1 + \nu \cos 2\theta) \partial_y^2 \psi. \quad (\text{S.19})$$

Discretizing time, we implement the trapezoidal rule for the diffusion term and keep the last nonlinear term explicit:

$$(\theta_{n+1} - \theta_n)/dt = \frac{1}{2A} (\partial_y^2 \theta_{n+1} + \partial_y^2 \theta_n) - \frac{1}{2} (1 + \nu \cos 2\theta_n) \partial_y^2 \psi_n, \quad (\text{S.20})$$

where  $dt$  is the time step and the subscript  $n$  denotes the current time iteration.

We use Eq. (S.16), which still holds, to compute  $\partial_y^2 \psi_n$ :

$$\partial_y^2 \psi_n = \frac{S(\sin 2\theta_n - \sin 2\theta_0) - \frac{R}{A} \partial_y^2 \theta_n}{2 + \frac{R\nu^2}{2} \sin^2 2\theta_n}. \quad (\text{S.21})$$

where  $\partial_y^2 \theta = -\mathcal{F}^{-1}[k^2 \hat{\theta}]$ , with  $\hat{\theta} = \mathcal{F}[\theta]$  denoting the Fourier transform.

At last, we solve Eq. (S.20) in Fourier space:

$$\hat{\theta}_{n+1} = \left(1 + \frac{dt}{2A} k^2\right)^{-1} \left( \left(1 - \frac{dt}{2A} k^2\right) \hat{\theta}_n - \frac{dt}{2} \mathcal{F}[(1 + \nu \cos 2\theta_n) \partial_y^2 \psi_n] \right). \quad (\text{S.22})$$

In our MATLAB script, we use  $N=1024$  gridpoints to span the range  $(0 : 1 - 1/N)$ , set  $dt = 0.005$ , and implement the 2/3 anti-aliasing rule prior to each real-space multiplication.

Our dynamical simulations are shown to converge on the predicted steady states (see Movies 1–4). In Fig. S.2, we further demonstrate the initial agreement with the predicted growth rate of linear perturbations about the quiescent state.

### S.6. MOVIE CAPTIONS

MOVIE 1. Relaxation onto the stable splay state (a1) in the contractile case. Black curve represents the time integration of Eq. (S.19), with parameters fixed as in Fig. 2(a). The initial condition was set to the dashed magenta curve (a2) with a small perturbation:  $\delta\theta = -0.01 \cos(2\pi y)$ .

MOVIE 2. Relaxation onto the quiescent state  $\theta = 0$  in the contractile case. Black curve represents the time integration of Eq. (S.19), with parameters fixed as in Fig. 2(a). The initial condition was set to the dashed magenta curve (a2) with a small perturbation:  $\delta\theta = 0.01 \cos(2\pi y)$ .

MOVIE 3. Relaxation onto the stable bend state (b1) in the extensile case. Black curve represents the time integration of Eq. (S.19), with parameters fixed as in Fig. 2(b). The initial condition was set to the quiescent state  $\theta = \pi/2$  with a small perturbation:  $\delta\theta = 0.01 \cos(2\pi y)$ .

MOVIE 4. Relaxation onto the stable splay state (b2) in the extensile case. Black curve represents the time integration of Eq. (S.19), with parameters fixed as in Fig. 2(b). The initial condition was set to the quiescent state  $\theta = 0$  with a small perturbation:  $\delta\theta = -0.01 \cos(2\pi y)$ .

## S.7. HAMILTONIAN ANALOGY

Here we provide more details on our mechanical analogy to the steady state problem. We consider the Hamiltonian  $H = \dot{\vartheta}^2/2 + U(\vartheta)$ , with the potential  $U$  defined in Eq. (8).

### A. Potential expansion

We gain insight by expanding  $U(\vartheta)$  about  $\vartheta = 0$  for  $S = -1$ . In the original  $\theta(y)$  problem, this corresponds to a splay pattern induced by a contractile stress.

$$U(\vartheta) = U_0 + a\vartheta^2 + b\vartheta^4 + \mathcal{O}(\vartheta^6), \quad (\text{S.23})$$

where

$$U_0 = U(\vartheta = 0), \quad a = \frac{(1 + \nu)}{2(4 + R(1 + \nu)^2)}, \quad b = -\frac{(4 + R + 16\nu + R\nu^2(3 + 4\nu))}{24(4 + R(1 + \nu)^2)^2}.$$

As noted in the main text,  $b$  changes sign precisely at  $\nu = \nu_{\pi/2}^*$ , where the supercritical to subcritical transition occurs. When  $a$  turns negative ( $\nu < -1$ ),  $U(\vartheta)$  becomes a double-well potential with the valleys corresponding to  $\cos \vartheta = 1/\nu$ .

### B. Computational trajectories

In Fig. S.3, we illustrate the potential, resulting trajectories, and their periods as functions of  $H$  for various values of negative  $\nu$ . In essence, this figure is a more detailed version of Fig. 3.

In the contractile case ( $S = -1$ , Fig. S.3(a)), top panels show  $U(\vartheta)$  (red curve) and a series of increasing  $H$  values spanning the range from  $U_0 = U(0)$  (dark blue) to  $U_{\max}$  (yellow). We use the ODE solver in Mathematica (**NDSolve** with default settings) to integrate Eq. (7) with the initial conditions:  $\vartheta(0) = 0$ ,  $\dot{\vartheta}(0) = \sqrt{2(H - U_0)}$ . The corresponding trajectories are shown in the second row of panels. We evaluate half of the pendulum period  $T$  by finding the second root of each trajectory. We then plot  $T$  as a function of  $H$  in the lower panels.

In the extensile case ( $S = +1$ , Fig. S.3(b)), top panels show  $U(\vartheta)$  (blue curve) and a series of increasing  $H$  values spanning the range from  $U_{\pi} = U(\pi)$  (dark blue) to  $U_{\max}$  (yellow). We integrate Eq. (7) with the initial conditions:  $\vartheta(0) = \pi$ ,  $\dot{\vartheta}(0) = \sqrt{2(H - U_{\pi})}$ . As in (a), these trajectories are shown in the second row of panels and their period  $T$  is plotted as a function of  $H$  in the lower panels.

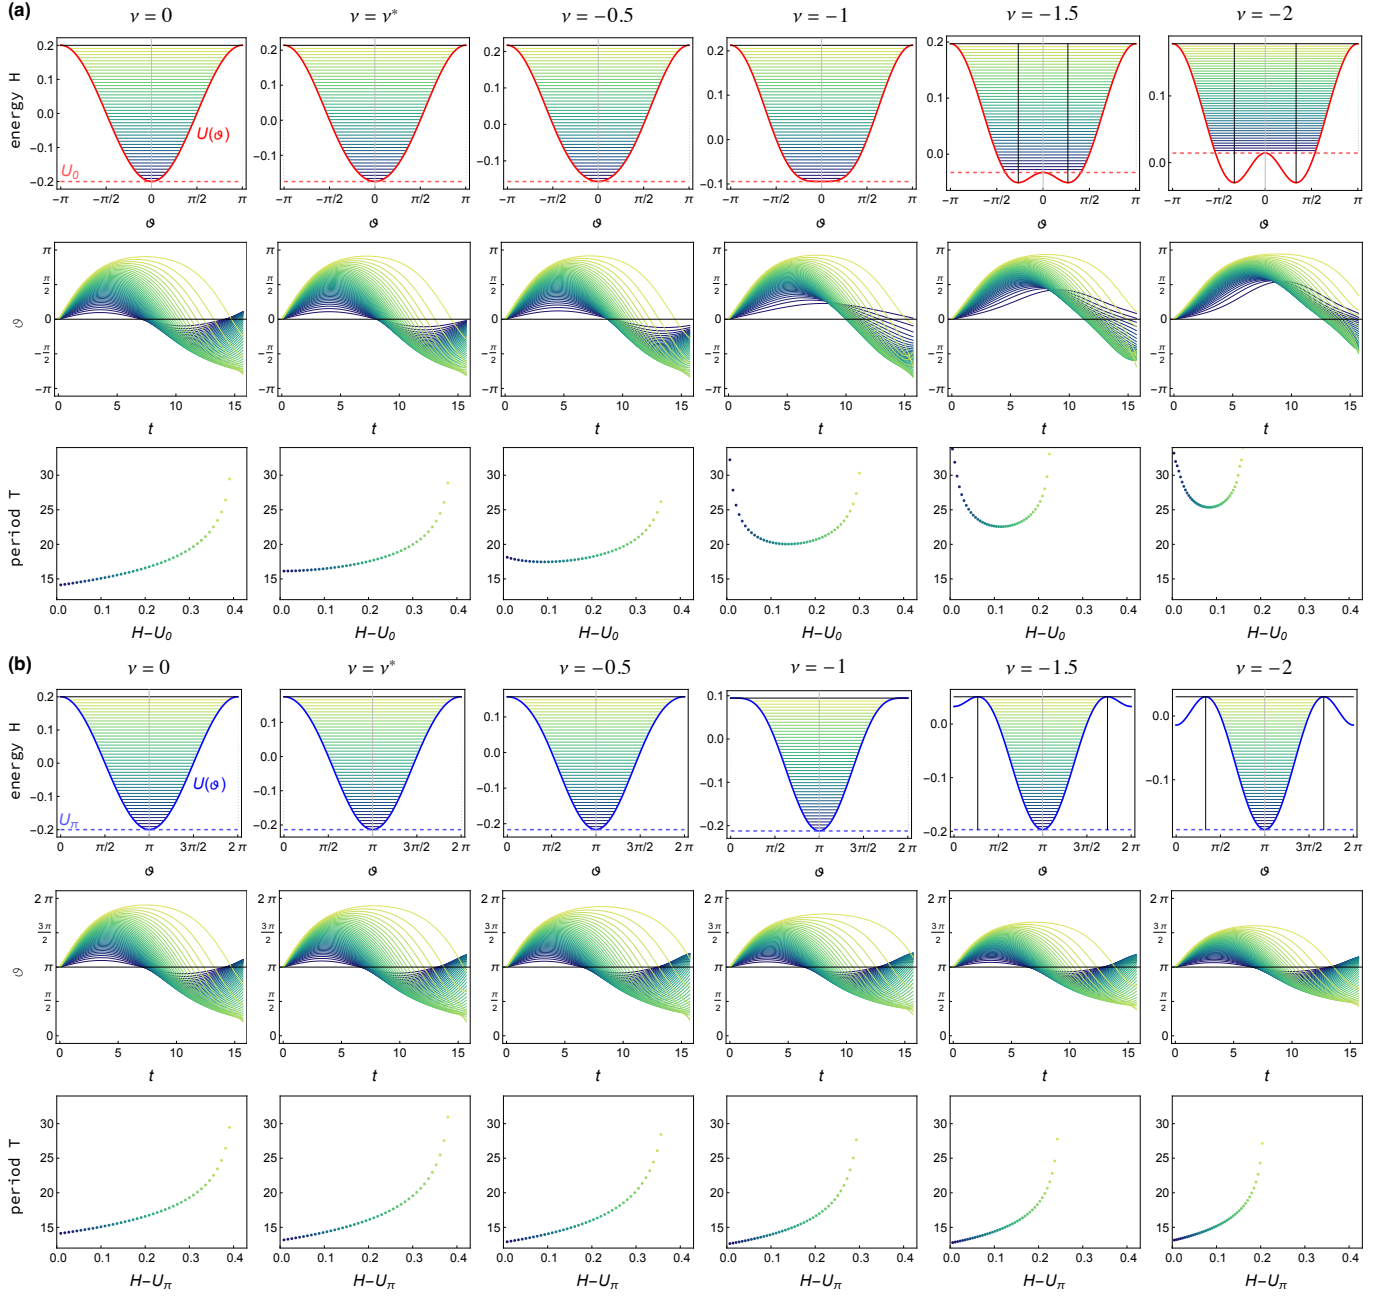

FIG. S.3. Hamiltonian analogy with  $S = -1$  (a) and  $S = +1$  (b). From left to right, we vary the flow-alignment parameter  $\nu$  while keeping  $R = 1$  fixed. The upper plots show the potential, Eq. (8), and the equi- $H$  lines corresponding to the  $\vartheta(t)$  trajectories plotted below. The period of these trajectories is plotted against the energy in the bottom panels.

- 
- [1] R. Alert, J.-F. Joanny, and J. Casademunt, Universal scaling of active nematic turbulence, *Nature Physics* **16**, 682 (2020).
  - [2] S. Edwards and J. Yeomans, Spontaneous flow states in active nematics: A unified picture, *Europhysics Letters* **85**, 18008 (2009).
  - [3] L. Giomi, M. J. Bowick, P. Mishra, R. Sknepnek, and M. Cristina Marchetti, Defect dynamics in active nematics, *Philosophical Transactions of the Royal Society A: Mathematical, Physical and Engineering Sciences* **372**, 20130365 (2014).
